# Supplementary material for: Velocity alignment explains Lagrangian irreversibility in turbulence
Source: arXiv:2503.12090 ancillary file (2025-03-15)
Supplement: Supplementary file 1 [file SI.pdf]

# Supplementary information: Velocity alignment explains Lagrangian irreversibility in turbulence

Ron Shnapp

Here, additional statistical information is shown regarding the backward and forward in time separation processes and the alignments of the separation and the relative velocity vectors. In Fig. 1 the probability distribution functions (PDFs) of the forward and backward distance between pairs are shown for three time values using two different normalization factors: the Kolmogorov length and the root mean squared (RMS) separation at each time. For all times shown, the separation is shown to have more extreme values of the separation in the backward as compared to the forward separation process (namely, more pairs have lower and higher values of the separation at fixed times in the backward separation). Nevertheless, as the RMS is more sensitive to the higher values of the distributions, only the faster separation of pairs is noticeable in the averaging leading to faster pair dispersion in the backward in time direction. Therefore, the backward separation process is not only faster, but also more intermittent that the forward separation.

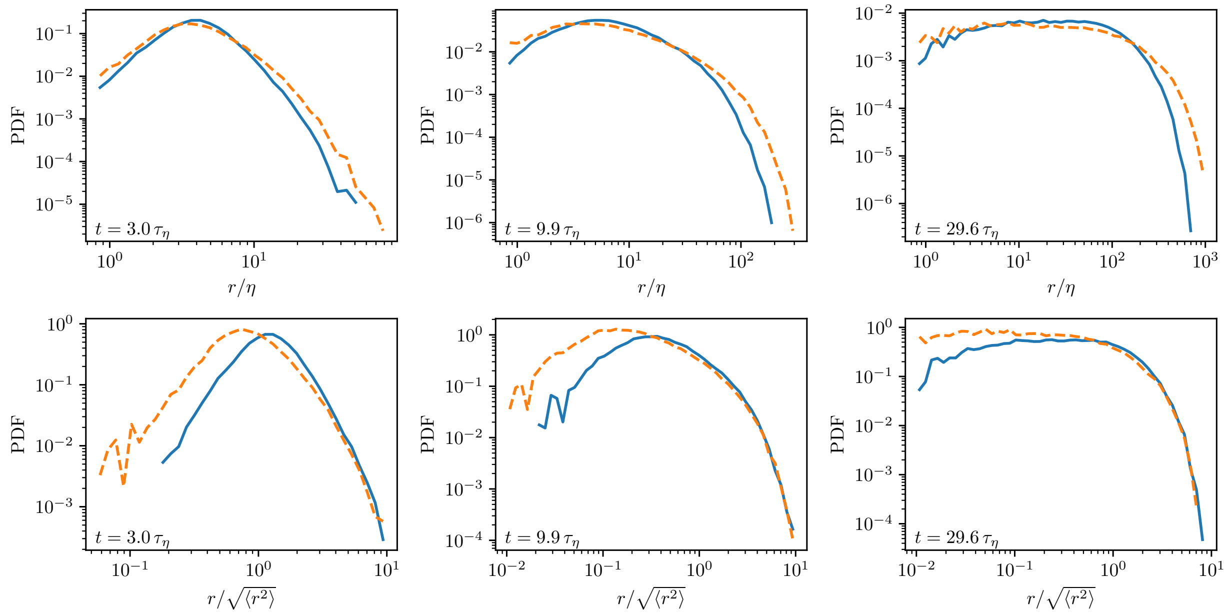


Figure 1: The distributions of the separation, backward and forward in time. Top row is normalized using the Kolmogorov scale, while the bottom row is normalized using the rms of the distribution at each time. Three time values are show as indicated on each sub-figure.

In Fig. 1 the PDF of $\theta$ is shown as a function of time for the backward and forward cases. The process is seen to initiate with $\theta$ distributions close to the uniform distribution case, and very quickly attain the

biased distributions that correspond to the inertial range. The time for the transition on the order of the eddy turnover time scale at the initial separation value, $\tau_b$.

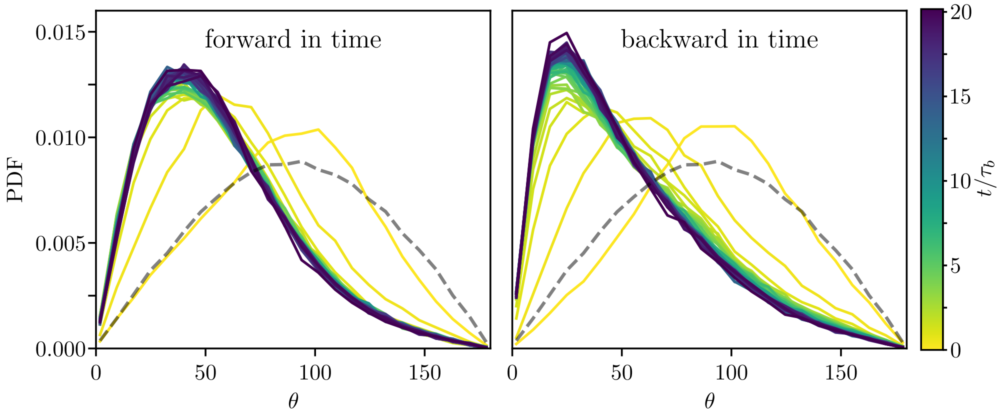


Figure 2: The distributions of the pair dispersion angle backward and forward in time, shown at various times along the separation process. Dashed lines show a uniform, random distribution of alignments between two vectors.

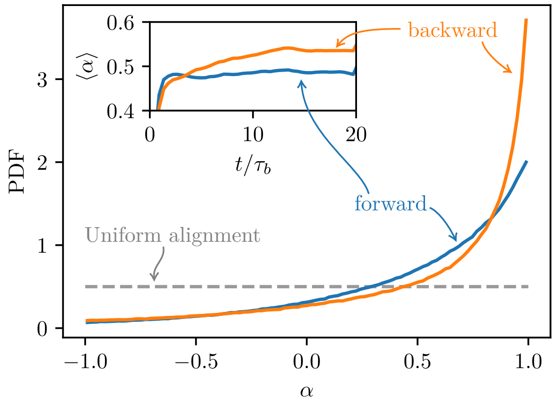


Figure 3: The distribution of the alignment projection between the separation and the relative velocity vectors, $\alpha = \cos(\theta)$, and its mean value shown in the inset. Data shown for the forward and backward separation cases and a dashed line indicates a uniform random distribution case.

Lastly, the PDF of the projection factor, $\alpha = \cos(\theta)$ is shown in Fig. 3 for both forward and backward in time directions and averaged across the inertial range, $t > 6\tau_b$. Also shown is the mean values shown as a function of time. Due to the biased distribution of $\theta$ towards aligned values $< 90°$, the projection, $\alpha = \cos(\theta)$, is biased towards higher values $\cos(\theta) > 0$. Furthermore, the projection is higher for the backward in time separation process, which eventually supports the Lagrangian irreversibility, as shown in the main text of the paper.
